# Supplementary material for: DeepSight: An All-in-One LM Safety Toolkit
Source: arXiv:2602.12092 source file (2026-02-12)
Supplement: Supplementary file 1 [file appendix.tex]

\section{Appendix: Examples of code}\label{sec:appendix}

Our proposed

\subsection{Configuration}
